# Supplementary material for: Transformers in Self-Supervised Monocular Depth Estimation with Unknown Camera Intrinsics
Source: arXiv:2202.03131 source file (2022-02-07)
Supplement: Supplementary file 1 [file appendix.tex]

\section{Appendix}
\label{sec:appendix}

\begin{table*}[t]
    %\centering
\resizebox{\linewidth}{!}{
\begin{tabular}{|l|c|c|c|c|}
\hline
Operation             & Input size                      & Output size                       & Function                                                          & \begin{tabular}[c]{@{}c@{}}Parameters\\ (DN3, DN6, DN9, DN12, PN)\end{tabular} \\ \hline
Read                  & $(N_p + 1) \times N_D$          & $N_p \times N_D$                  & Drop readout token                                                & $-$                                                                            \\
Concatenate           & $N_p \times N_D$                & $N_D \times H / p \times W / p$   & Transpose and Unflatten                                           & $-$                                                                            \\
Pointwise Convolution & $N_D \times H / p \times W / p$ & $N_c \times H / p \times W / p$   & $N_c$ channels                                                    & $N_c=[96, 768, 1536, 3072, 2048]$                                              \\
Strided Convolution   & $N_c \times H / p \times W / p$ & $N_c \times H / 2p \times W / 2p$ & $k \times k$ convolution, Stride$=2$, $N_c$ channels, padding$=1$ & $k=[-, -, -, 3, -]$                                                            \\
Transpose Convolution & $N_c \times H / p \times W / p$ & $N_c \times H / s \times W / s$   & $p/s \times p/s$ deconvolution, stride$=p/s$, $N_c$ channels      & $s=[4, 2, -, -, -]$                                                            \\ \hline
\end{tabular}
}
    \caption{Reassemble}
    \label{tab:reassemble}
\end{table*}

\begin{table}[t]
    %\centering
\begin{tabular}{|c|}
\hline
Layers                                                                            \\ \hline
$32$ $3 \times 3$ \textit{Convolutions}, stride=$1$, padding$=1$ \\
\textit{ReLU}                                                    \\
\textit{Bilinear Interpolation} to upsample by $2$                \\
$32$ \textit{}{Pointwise Convolutions}                                                   \\
\textit{Sigmoid}                                                 \\ \hline
\end{tabular}
    \caption{Head modules}
    \label{tab:heads}
\end{table}
